# Supplementary material for: Generate, Discriminate and Contrast: A Semi-Supervised Sentence Representation Learning Framework
Source: arXiv:2210.16798 source file (2022-10-30)
Supplement: Supplementary file 1 [file appendix.tex]

\clearpage

\appendix

\section{Synthetic data samples}
In this section, we gives more synthetic data samples in Table~\ref{tab:full_gen_samples}. For each input sentences, we gives two samples using over-generation.

\input{tables/full_gen_samples}
